# Supplementary material for: An improved coarse-grained model of solvation and the hydrophobic effect
Source: arXiv:1010.5750 source file (2010-10-27)
Supplement: Supplementary file 1 [file Supplementary.pdf]

# Supplementary Data for "An improved coarse-grained model of solvation and the hydrophobic effect"

## 1 Model hydrophobic plate coordinates

The supplementary file `hydrophobic_plate.dat` includes the coordinates of the oily sites in the model hydrophobic plate used in the paper. This plate, first used in J. Phys. Chem. B **114**, 1632 (2010), was made by recording the positions of all water oxygens inside a $24 \times 24 \times 3\,\text{Å}^3$ subvolume of an SPC/E water simulation in the $NVT$ ensemble, with temperature $T = 298\,\text{K}$. The simulation box included a vapor bubble to ensure that the liquid water was at coexistence with its vapor.

The first non-commented line of the file specifies the number of oily sites in the plate (52) and the Lennard-Jones $\sigma$ (in Å) and $\epsilon$ (in kcal/mol) parameters that describe the interaction between an oily-site and an SPC/E water oxygen atom. All subsequent lines are $(x, y, z)$ coordinates of the oily sites, in Å.

## 2 Precalculated values for $\chi_{ab}$

The supplementary file `NartenLevy_T25C_chi_ab_lambda_1.dat` includes $\chi_{ab}$ values for water at temperature $T = 298\,\text{K}$ and pressure $p = 1\,\text{atm}$, calculated as described in the Appendix. Let $\mathbf{d}$ be the vector from the center of cell $a$ to the center of cell $b$, measured in units of $\lambda_f$. Since the $\chi_{ab}$ matrix has translational symmetry, we need only specify its non-zero values of its elements for all different vectors $\mathbf{d}$. Additionally, since the matrix

also has rotational and reflection symmetry, we only include the values for vectors $\mathbf{d}$ whose coordinates are non-negative and non-decreasing. Each line in the file gives the coordinates of $\mathbf{d}$, the corresponding value of $\chi_{ab}$ and an estimate of the error in evaluating the integral that determines its value. Note that the experimental error in determining the structure factor is a much larger source of error.

Similarly, the supplementary file `SPCE_1atm_298K_chi_ab_lambda_1.dat` summarizes the results of calculating $\chi_{ab}$ from a 1 ns NPT simulation of a $30 \times 30 \times 30\,\text{Å}^3$ box of SPC/E water created with GROMACS 4 (an initial 100 ps equilibration period is ignored). The format is unchanged from above, except that the error quoted is statistical, due to the use of a finite trajectory, and not an integration error.

# 3 Water number distributions

Figures 1–3 show the $P_V(N)$ distributions for the confinement simulations described in the main text, from $d = 7$ Å to $d = 11$ Å in steps of 1 Å, and with $\eta = 0.0$, 0.5 and 1.0. For clarity, we omit the additional intervening $P_V(N)$ distribution used to construct the phase diagram in the main text. No qualitatively different features are present in these distributions.

For the distributions calculated in explicit SPC/E water, we equilibrated the waters in the absence of an umbrella potential for 1 ns. We then made several independent 1 ns umbrella runs with $\tilde{N}_0$ values spaced out at every 4 waters. We ignored the first 100 ps of each run, where $\tilde{N}$ quickly tended to $\tilde{N}_0$. In several umbrella runs near the free energy barriers, equilibration was clearly not complete in 100 ps, as judged by abrupt transition of the mean value of $\tilde{N}$ far into the production phase of the runs. For these few umbrellas, we ran an extra 4 ns, and used only this extra portion of the trajectories when gathering statistics.

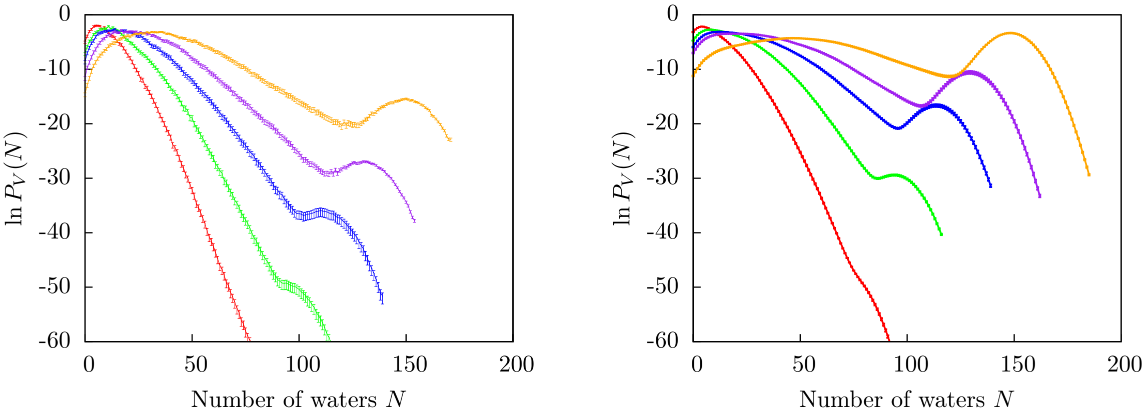


SPC/E, $\eta = 0.0$ Coarse-grained model, $\eta = 0.0$

Figure 1: $P_V(N)$ distributions for probe volumes between confined plates with attractive strength $\eta = 0.0$. The plate separations range from $d = 7\,\text{Å}$ (red) to $d = 11\,\text{Å}$ (orange). See Figure 3 for full color code

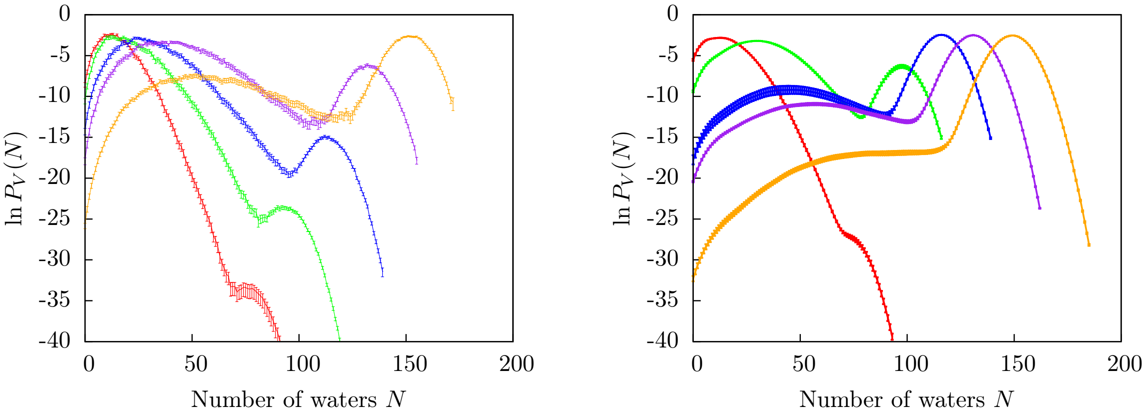


SPC/E, $\eta = 0.5$ Coarse-grained model, $\eta = 0.5$

Figure 2: $P_V(N)$ distributions for probe volumes between confined plates with attractive strength $\eta = 0.5$. The plate separations range from $d = 7\,\text{Å}$ (red) to $d = 11\,\text{Å}$ (orange). See Figure 3 for full color code

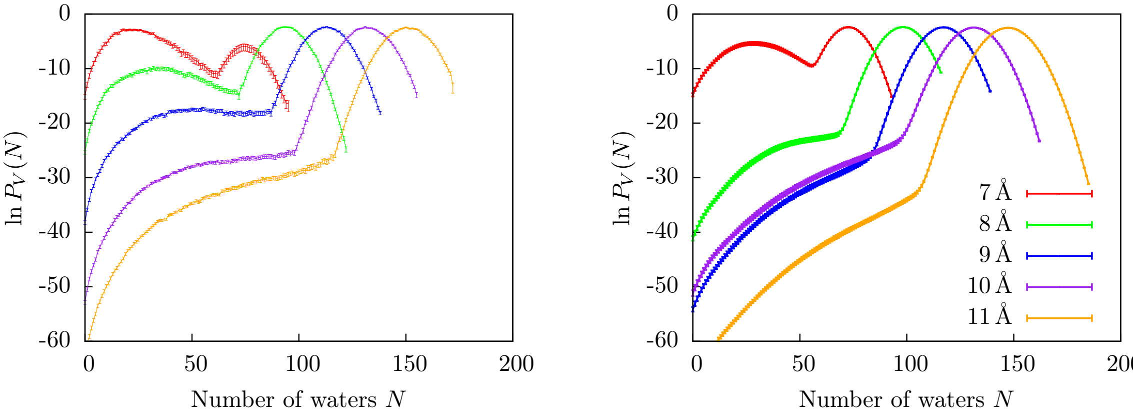


SPC/E, $\eta = 1.0$

Coarse-grained model, $\eta = 1.0$

Figure 3: $P_V(N)$ distributions for probe volumes between confined plates with attractive strength $\eta = 1.0$. The plate separations range from $d = 7$ Å (red) to $d = 11$ Å (orange).
